# Supplementary material for: CoDS: Robust Collaborative Perception via Expert-driven Detection and BEV Segmentation
Source: arXiv:2608.14085 source file (2026-08-14)
Supplement: Supplementary file 1 [file X_suppl.tex]

\appendix

\section{More Implementation Details}
\subsection{Datasets}

We validate our CoDS on two datasets: OPV2V~\cite{10-attfuse} and V2V4Real~\cite{41-v2v4real}. 

\textbf{OPV2V} is a large-scale open simulated dataset for V2V cooperative perception, built upon the CARLA~\cite{42-carla} simulator and the OpenCDA~\cite{43-opencda} co-simulation framework. It covers 73 diverse driving scenes across 9 towns, comprising 11,464 multi-vehicle perception frames and 232,913 annotated 3D bounding boxes. Notably, OPV2V provides dual-task annotations for both 3D object detection and BEV semantic segmentation, making it a well-established benchmark for cooperative 
multi-task perception research. 

\textbf{V2V4Real} is the first large-scale real-world multimodal dataset for V2V cooperative perception, collected by two sensor-equipped vehicles driving together through diverse real-world scenarios. It spans a driving area of approximately 410\,km and contains 20K LiDAR frames, 40K RGB 
frames, and 240K annotated 3D bounding boxes across five object categories. While V2V4Real offers a rigorous testbed for evaluating generalization under real-world conditions, it does not provide BEV semantic segmentation annotations. Therefore, we evaluate the segmentation branch of CoDS exclusively on OPV2V, and report detection performance on both datasets.

\subsection{Metrics}

For 3D object detection, we adopt Average Precision~(AP) as the primary evaluation metric, reported at IoU thresholds of 0.3, 0.5, and 0.7. For BEV semantic 
segmentation, we employ mean Intersection over Union~(mIoU) averaged over all semantic categories, including dynamic objects, road, and lane markings. For efficiency evaluation, we report parameter count~(Params.), floating-point operations~(FLOPs), and average GPU memory consumption during inference~(Mem.).

\subsection{Training Configuration}
The point cloud is voxelized at a resolution of $0.4 \times 0.4 \times 4.0$\,m with
at most 32 points per voxel, over a LiDAR range of $x \in [-140.8, 140.8]$\,m and
$y \in [-51.2, 51.2]$\,m. The V2V communication range is fixed at 70\,m with at most
5 collaborating vehicles per frame. Anchors are defined with dimensions
$l{=}3.9$\,m, $w{=}1.6$\,m, $h{=}1.56$\,m at two orientations ($0^\circ$, $90^\circ$),
with positive/negative IoU thresholds of 0.6/0.45 for assignment and NMS threshold
of 0.15 at inference, retaining at most 100 detections per frame.

All models are optimized with Adam~\cite{44-adam} at an initial learning rate of
$2 \times 10^{-3}$ and weight decay of $10^{-4}$, with a multi-step decay of
$0.1\times$ at epochs 10 and 20, trained for 30 epochs with batch size 2.
Data augmentation includes random flipping, rotation within $[-45^\circ, 45^\circ]$,
and scaling in $[0.95, 1.05]$.
All experiments are conducted on two NVIDIA RTX 4090 GPUs.


\section{More Quantitative Results}

% 表格1：检测结果
\begin{table}[!t]
\centering
\caption{Detection performance when integrating CoDS with different fusion strategies on OPV2V.
Rows labeled \textit{Improvement} report the absolute gain of each ``w/ CoDS'' variant
over its corresponding backbone.}
\label{tab:plug_det}
\resizebox{0.9\columnwidth}{!}{%
\begin{tabular}{l | ccc}
\hline
\textbf{Method} & \textbf{AP@0.3} & \textbf{AP@0.5} & \textbf{AP@0.7} \\
\hline
1. AttFuse~\cite{10-attfuse}       & 89.94 & 89.41 & 83.65 \\
2. AttFuse w/ CoDS                 & 94.64 & 94.05 & 86.88 \\
\cellcolor{gray!10}\textit{Improvement (2-1)}         & \cellcolor{gray!10}\textit{+4.70} & \cellcolor{gray!10}\textit{+4.64} & \cellcolor{gray!10}\textit{+3.23} \\
\hline
1. CoAlign~\cite{11-coalign}       & 89.27 & 88.85 & 82.73 \\
2. CoAlign w/ CoDS                 & 93.29 & 92.63 & 85.83 \\
\cellcolor{gray!10}\textit{Improvement (2-1)}         & \cellcolor{gray!10}\textit{+4.02} & \cellcolor{gray!10}\textit{+3.78} & \cellcolor{gray!10}\textit{+3.10} \\
\hline
1. CoSDH~\cite{13-cosdh}           & 91.06 & 90.54 & 82.48 \\
2. CoSDH w/ CoDS                   & 93.13 & 92.35 & 85.23 \\
\cellcolor{gray!10}\textit{Improvement (2-1)}         & \cellcolor{gray!10}\textit{+2.07} & \cellcolor{gray!10}\textit{+1.81} & \cellcolor{gray!10}\textit{+2.75} \\
\hline
\end{tabular}
}
\end{table}


% 表格2：分割结果
\begin{table}[!t]
\centering
\caption{BEV segmentation performance when integrating CoDS with different fusion strategies on OPV2V. Rows labeled \textit{Improvement} report
the absolute gain of each ``w/ CoDS'' variant over its corresponding backbone.}
\label{tab:plug_seg}
\resizebox{0.85\columnwidth}{!}{%
\begin{tabular}{l | ccc}
\hline
\textbf{Method} & \textbf{Dynamic} & \textbf{Road} & \textbf{Lane} \\
\hline
1. AttFuse~\cite{10-attfuse}       & 71.20 & 63.97 & 48.08 \\
2. AttFuse w/ CoDS                 & 76.47 & 69.38 & 55.19 \\
\cellcolor{gray!10}\textit{Improvement (2-1)}         & \cellcolor{gray!10}\textit{+5.27} & \cellcolor{gray!10}\textit{+5.41} & \cellcolor{gray!10}\textit{+7.11} \\
\hline
1. CoAlign~\cite{11-coalign}       & 71.57 & 63.88 & 48.33 \\
2. CoAlign w/ CoDS                 & 74.76 & 66.55 & 51.47 \\
\cellcolor{gray!10}\textit{Improvement (2-1)}         & \cellcolor{gray!10}\textit{+3.19} & \cellcolor{gray!10}\textit{+2.67} & \cellcolor{gray!10}\textit{+3.14} \\
\hline
1. CoSDH~\cite{13-cosdh}           & 72.54 & 62.35 & 46.31 \\
2. CoSDH w/ CoDS                   & 74.14    & 66.23 & 50.98 \\
\cellcolor{gray!10}\textit{Improvement (2-1)}         & \cellcolor{gray!10}\textit{+1.60}     & \cellcolor{gray!10}\textit{+3.88} & \cellcolor{gray!10}\textit{+4.67} \\
\hline
\end{tabular}
}
\end{table}

\subsection{Scalability to Different Fusion Strategies}
To investigate the scalability of CoDS across different collaborative fusion strategies, we integrate it with AttFuse~\cite{10-attfuse}, CoAlign~\cite{11-coalign}, and
CoSDH~\cite{13-cosdh}, and evaluate the resulting performance changes on OPV2V, with results reported in Table~\ref{tab:plug_det} and Table~\ref{tab:plug_seg}.
CoDS consistently improves both detection and segmentation across all three fusion backbones, indicating that the proposed reliability modeling and multi-task interaction mechanisms are not sensitive to the specific form of the underlying fusion strategy.
Notably, the most substantial gains are observed when CoDS is built upon AttFuse, which we attribute to the attention-based fusion mechanism of AttFuse being more
amenable to joint modeling with the Collaborative Reliability Map. Accordingly, we adopt AttFuse as the default fusion strategy for CoDS in all main
experiments.

% 表格
\begin{table*}[!t]
\centering
\caption{Effect of BTCI under increasing Gaussian localization noise on OPV2V.
The column headers denote the injected pose noise level
(translation in meters\,/\,rotation in degrees).
``w/o BTCI'' denotes the model without the Bidirectional Task Complementary
Interaction module. Best results are in \textbf{bold}.}
\label{tab:btci_noise}
\resizebox{\textwidth}{!}{%
\begin{tabular}{c | cccc | cccc | cccc | cccc}
\hline
\multirow{2}{*}{\textbf{Method}} 
& \multicolumn{4}{c|}{\textbf{0/0}} 
& \multicolumn{4}{c|}{\textbf{0.2/0.2}} 
& \multicolumn{4}{c|}{\textbf{0.4/0.4}} 
& \multicolumn{4}{c}{\textbf{0.6/0.6}} \\
\cline{2-17}
& \textbf{AP@0.5} & \textbf{Dynamic} & \textbf{Road} & \textbf{Lane}
& \textbf{AP@0.5} & \textbf{Dynamic} & \textbf{Road} & \textbf{Lane}
& \textbf{AP@0.5} & \textbf{Dynamic} & \textbf{Road} & \textbf{Lane}
& \textbf{AP@0.5} & \textbf{Dynamic} & \textbf{Road} & \textbf{Lane} \\
\hline
w/o BTCI
& 93.56 & 75.82 & 67.44 & 53.11
& 92.93 & 75.16 & 66.86 & 52.26
& 89.00 & 73.82 & 65.88 & 50.73
& 80.93 & 72.27 & 64.76 & 49.21 \\
Ours
& \textbf{94.05} & \textbf{76.47} & \textbf{69.38} & \textbf{55.19}
& \textbf{93.51} & \textbf{75.65} & \textbf{68.65} & \textbf{54.01}
& \textbf{89.61} & \textbf{74.15} & \textbf{67.53} & \textbf{52.11}
& \textbf{81.29} & \textbf{72.51} & \textbf{66.41} & \textbf{50.35} \\
\hline
\end{tabular}
}
\end{table*}

\subsection{Effect of BTCI under Localization Noise}
To further examine the contribution of BTCI under noisy conditions, we compare models with and without BTCI across increasing levels of Gaussian localization noise,
with results reported in Table~\ref{tab:btci_noise}.
Under the noise-free setting~(0/0), BTCI consistently improves both detection and segmentation, with the most notable gains on Road and Lane IoU of 1.94 and 2.08 points, respectively, confirming the benefit of injecting detection boundary responses as contour priors for segmentation. More importantly, BTCI maintains a consistent performance advantage over the w/o BTCI
baseline across all noise levels, demonstrating that the bidirectional injection of detection boundary and segmentation road priors provides stable cross-task
complementary compensation regardless of noise intensity. These results confirm that explicitly modeling inter-task complementarity is an effective strategy for enhancing robustness in low-reliability collaborative fusion scenarios.

\subsection{Source of performance gains.} 
We design two parameter-matched variants to isolate the effect of semantic routing: (1) Single Expert (equal capacity, no routing); (2) Random Routing (MoE with random gating). As shown in Table~\ref{tab:gains}, both variants underperform our S-MoE, especially on Lane IoU, where S-MoE outperforms Single Expert by 10.56 and Random Routing by 10.69. This confirms gains stem from reliability-guided semantic routing, not from added capacity or complexity.
\begin{table}[ht]
\centering
\caption{Source of performance gains. Best in \textbf{bold}.}
\label{tab:gains}
\resizebox{0.9 \columnwidth}{!}{%
\begin{tabular}{l|c|ccccc}
\toprule
\textbf{Variant} & \textbf{AP@0.5} & \textbf{Dynamic} & \textbf{Road} & \textbf{Lane} \\
\midrule
Single Expert       & 91.99 & 73.60 & 66.57 & 44.63 \\
Random Routing      & 89.14 & 70.93 & 64.58 & 44.50 \\
S-MoE (Ours)   & \textbf{94.05} & \textbf{76.47} & \textbf{69.38} & \textbf{55.19} \\
\bottomrule
\end{tabular}
}
\end{table}

\subsection{Routing init sensitivity.}
We ablate $\alpha_{det}$ and $\alpha_{seg}$ (Table~\ref{tab:Routing}). The best configuration is 0.70/0.45, achieving top scores across all metrics. This shows detection benefits from a stronger prior for sparse objects, while segmentation prefers learned routing. Other settings cause clear drops, indicating the need for a balanced but detection-skewed initialization.

\begin{table}[ht]
\centering
\caption{Routing init sensitivity. Best in \textbf{bold}.}
\label{tab:Routing}
\resizebox{0.85\columnwidth}{!}{%
\begin{tabular}{l|c|ccc}
\toprule
$\alpha_{det}$/$\alpha_{seg}$ & {AP@0.5} & {Dynamic} & {Road} & {Lane} \\
\midrule
0.50 / 0.50          & 92.63          & 74.07          & 66.29          & 44.56          \\
0.65 / 0.45          & 92.10          & 72.58          & 68.02          & 48.15          \\
\textbf{0.70 / 0.45} & \textbf{94.05} & \textbf{76.47} & \textbf{69.38} & \textbf{55.19} \\
0.80 / 0.50          & 92.63          & 73.15          & 68.43          & 45.79          \\
\bottomrule
\end{tabular}
}
\end{table}


\subsection{Joint perturbation experiment.} We further evaluate CoDS under joint perturbations combining pose noise and communication latency simultaneously. As shown in Table~\ref{tab:joint_perturbation}, CoDS consistently outperforms all baselines across all three settings. Notably, the performance gap grows as perturbation intensity increases, with CoDS maintaining particularly strong advantages at AP@0.5 and Dynamic IoU under the most severe condition (600\,ms, 0.6\,m, 0.6$^\circ$). These results confirm that CoDS effectively handles concurrent multi-source disturbances, demonstrating its practical robustness for real-world deployment.

\begin{table}[ht]
\centering
\caption{Joint perturbation experiment. Best in \textbf{bold}.}
\label{tab:joint_perturbation}
\resizebox{\columnwidth}{!}{%
\begin{tabular}{l|ccc|ccc|ccc}
\toprule
\multirow{2}{*}{{Method}}
  & \multicolumn{3}{c|}{$(0\,\text{ms},\;0\,\text{m},\;0^\circ)$}
  & \multicolumn{3}{c|}{$(0\text{--}300\,\text{ms},\;0.3\,\text{m},\;0.3^\circ)$}
  & \multicolumn{3}{c}{$(0\text{--}600\,\text{ms},\;0.6\,\text{m},\;0.6^\circ)$} \\
\cmidrule(lr){2-4}\cmidrule(lr){5-7}\cmidrule(lr){8-10}
 & AP@0.5 & AP@0.7 & Dyn. & AP@0.5 & AP@0.7 & Dyn. & AP@0.5 & AP@0.7 & Dyn. \\
\midrule
AttFuse &  89.41 & 83.65  & 71.20  & 75.29  & 50.28 & 65.33 & 55.56 & 33.10 & 60.64 \\
CoAlign &  88.85 & 82.73  & 71.57   & 74.13 & 48.86 & 64.99 & 54.35 & 31.92 & 59.74 \\
{Ours} & \textbf{94.05} & \textbf{86.88} & \textbf{76.47}  & \textbf{80.48}  & \textbf{51.71} & \textbf{67.61} & \textbf{59.81} & \textbf{34.90} & \textbf{62.18} \\
\bottomrule
\end{tabular}
}
\end{table}

\subsection{More severe positioning noise.} We further evaluate CoDS under more extreme localization errors, extending the noise level up to $(1.2\,\text{m},\;1.2^\circ)$. As reported in Table~\ref{tab:severe_noise}, CoDS consistently surpasses all baselines across every noise setting. Notably, as the perturbation intensifies, the performance gap between CoDS and the baselines widens substantially—at the most challenging condition $(1.2\,\text{m},\;1.2^\circ)$, our method outperforms AttFuse by 6.77 points in AP@0.3. These results strongly demonstrate the  robustness of CoDS under severe positioning disturbances.

\begin{table}[ht]
\centering
\caption{More severe positioning noise. Best in \textbf{bold}.}
\label{tab:severe_noise}
\resizebox{\columnwidth}{!}{%
\begin{tabular}{l|c|c|c|c|c}
\toprule
Method & $(0\,\text{m},\;0^\circ)$& $(0.3\,\text{m},\;0.3^\circ)$ & $(0.6\,\text{m},\;0.6^\circ)$ & $(0.9\,\text{m},\;0.9^\circ)$ & $(1.2\,\text{m},\;1.2^\circ)$ \\
\midrule
AttFuse  & 89.94  & 89.73   & 86.56   & 72.61 & 61.13 \\
CoAlign  & 89.27 & 89.07   & 86.39   & 72.25  &  60.39\\
{Ours} & \textbf{94.64} & \textbf{94.25} & \textbf{91.57} & \textbf{78.54} & \textbf{67.90} \\
\bottomrule
\end{tabular}
}
\end{table}


\subsection{Tasks complementarity under noise.}
We compare CoDS against single-task variants (Det-only and Seg-only) under pose noise to verify cross-task benefits. As shown in Table~\ref{tab:task_complementarity}, CoDS consistently outperforms both single-task counterparts across all noise levels. For example, at $(0.6\,\text{m}, 0.6^\circ)$, CoDS surpasses Det-only by 16.23 points in AP@0.5 and Seg-only by 10.15 points in Dynamic IoU. These results confirm that joint training effectively leverages task complementarity, yielding robust improvements even under severe noise.

\begin{table}[ht]
\centering
\caption{Tasks complementarity under noise. Best in \textbf{bold}.}
\label{tab:task_complementarity}
\resizebox{1.0\columnwidth}{!}{%
\begin{tabular}{l|cc|cc|cc}
\toprule
\multirow{2}{*}{Method} & \multicolumn{2}{c|}{$(0\,\text{m},\;0^\circ)$} & \multicolumn{2}{c|}{$(0.3\,\text{m},\;0.3^\circ)$} & \multicolumn{2}{c}{$(0.6\,\text{m},\;0.6^\circ)$} \\
 & AP@0.5 & Dynamic & AP@0.5 & Dynamic & AP@0.5 & Dynamic \\
\midrule
Det-only & 91.69 & {-} & {83.63} & {-} & {65.06} & {-} \\
Seg-only & {-} & 71.22 & {-} & {66.21} & {-} & {62.36} \\
Ours     & \textbf{94.05} & \textbf{76.47} & \textbf{92.33} & \textbf{74.93} & \textbf{81.29} & \textbf{72.51} \\
\bottomrule
\end{tabular}
}
\end{table}



\begin{figure*}[!t]
    \centering
    \includegraphics[width=\textwidth]{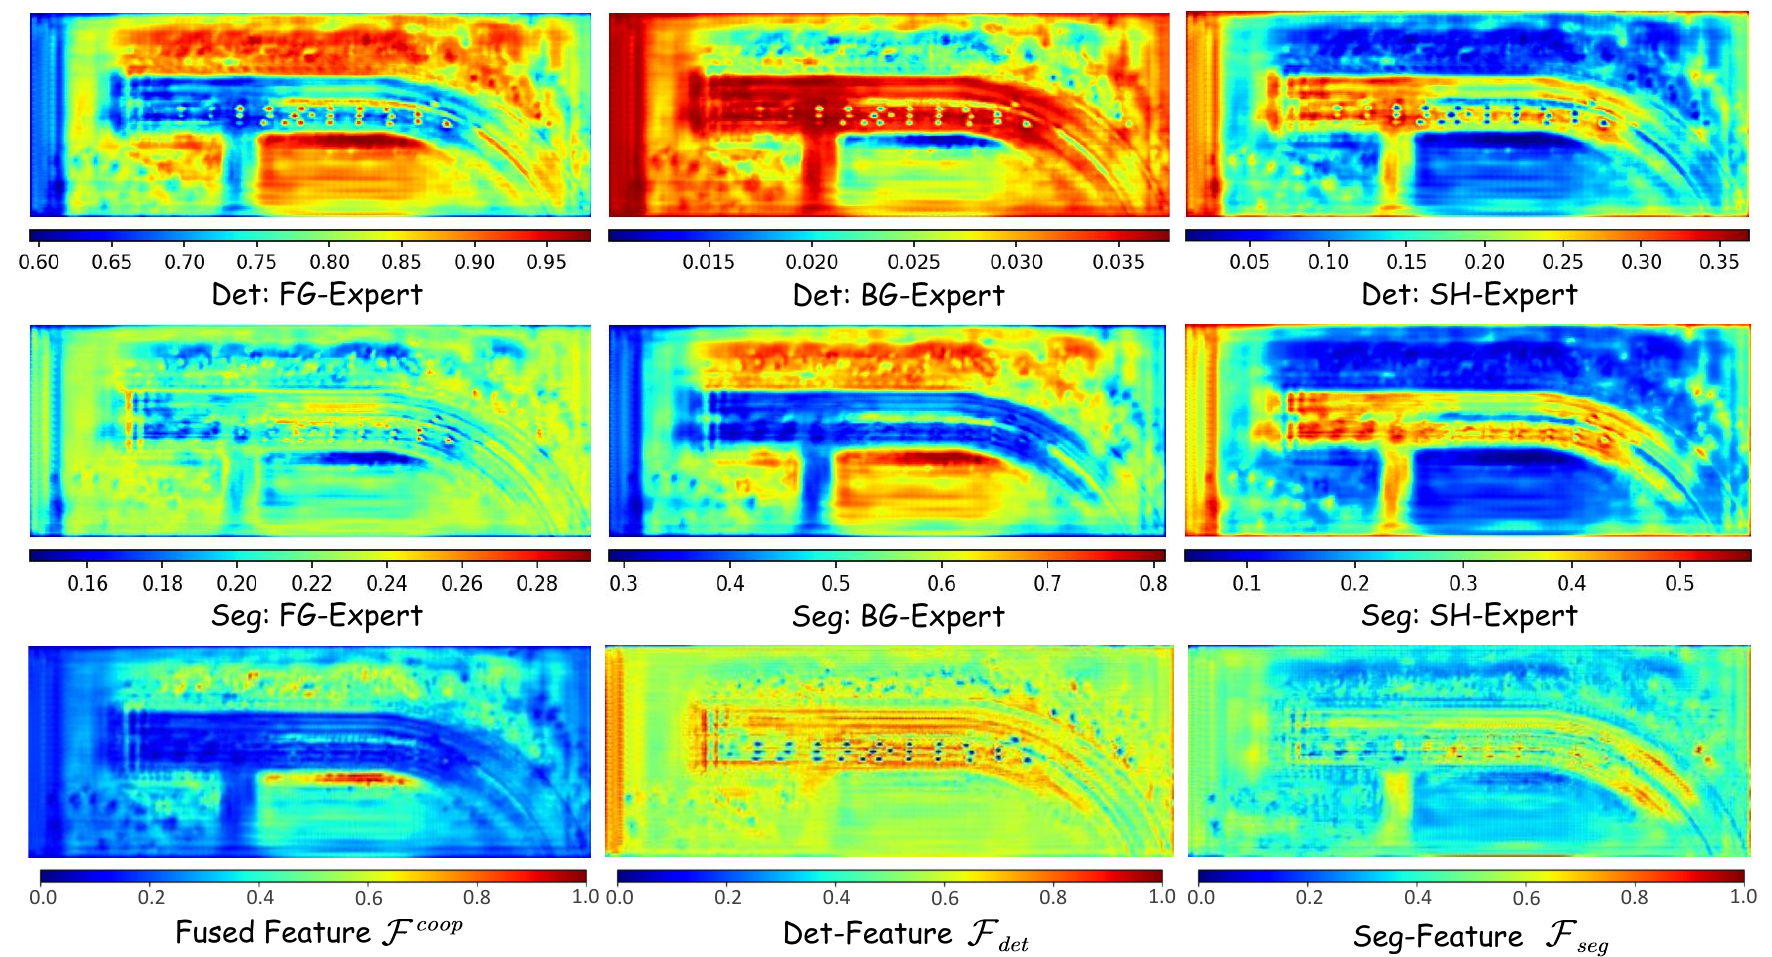}
    \caption{
    Visualization of expert activation maps under detection and segmentation tasks
    on OPV2V.
    \textbf{Top row}: activation maps of FG-Expert, BG-Expert, and SH-Expert for
    the detection task.
    \textbf{Middle row}: activation maps of FG-Expert, BG-Expert, and SH-Expert
    for the segmentation task.
    \textbf{Bottom row}: the collaborative fused feature $\mathcal{F}^{coop}$,
    the detection-specific feature $\mathcal{F}_{det}$, and the
    segmentation-specific feature $\mathcal{F}_{seg}$ produced by S-MoE.
    Warmer colors indicate higher activation values.
    }
    \Description{None.}
    \label{fig:expert_vis}
\end{figure*}

\section{More Qualitative Analysis}
\subsection{Expert Activation Visualization}
To further interpret the behavior of the S-MoE module, we visualize the activation maps of each expert under the detection and segmentation tasks, along with the collaborative fused feature $\mathcal{F}^{coop}$ and the resulting task-specific features $\mathcal{F}_{det}$ and $\mathcal{F}_{seg}$, as shown in Fig.~\ref{fig:expert_vis}. For the detection task, FG-Expert produces strong concentrated activations around
object regions, while BG-Expert dominates continuous road and lane structures in the segmentation task, confirming the role specialization learned by the routing
mechanism. Comparing $\mathcal{F}^{coop}$ with the task-specific outputs, S-MoE effectively disentangles the mixed collaborative representation: $\mathcal{F}_{det}$ sharpens object-region responses with suppressed background noise, while $\mathcal{F}_{seg}$ amplifies continuous road structural patterns, demonstrating that S-MoE successfully extracts differentiated task-specific features from spatially heterogeneous collaborative fused features.
